# Supplementary material for: Learning to Memorize in Neural Task-Oriented Dialogue Systems
Source: arXiv:1905.07687 source file (2019-05-19)
Supplement: Supplementary file 1 [file appendix1.tex]

\chapter{Appendix 1}
